# Supplementary material for: Fixed-Confidence Guarantees for Bayesian Best-Arm Identification
Source: arXiv:1910.10945 source file (2019-10-28)
Supplement: Supplementary file 1 [file app_future.tex]

\section{Future work}\label{app:future}

% In this paper, we provided a fixed-confidence analysis for \TTTS. It would also be meaningful to provide a fixed-budget analysis, in particular in some potential application scenario of \TTTS. For example, pure exploration bandit algorithms are widely used in \emph{hyper-parameter optimization} for machine learning~\citep{hoffman2014bayesgap,li2017hyperband,shang2019dttts}.
% 
% 
% Another important unsolved open question comes to the tuning of $\beta$. Indeed, if $\beta$ is set to $\beta^\star = \argmax_{\beta \in [0,1]} \Gamma_\beta^\star$, a $\beta$-optimal strategy is also optimal. In practice of course $\beta^\star$ is unknown and so far \TTTS cannot be asymptotically optimal without this knowledge. However, note that \cite{russo2016ttts} shows that $\Gamma^\star_{1/2} \geq \Gamma^{\star}/2$, which provides a near-optimal tuning of \TTTS. Obviously, proposing an satisfying online tuning of $\beta$ (other than the one proposed in the \TTTS paper) with provable fixed confidence guarantees is another avenue for future work.
% 
% There is another line of research that leverages a game theoretic point of view on the pure exploration setting, that explores a statistic-computation trade-off~\citep{menard2019lma,degenne2019solvinggame}. One open question is to investigate whether Thompson Sampling-based exploration can replace the current (complicated) optimistic approach.

% Finally, it is also interesting to know whether there exist better sampling methods, that can accelerate the procedure of sampling the challenger.
