# Supplementary material for: Fixed-Confidence Guarantees for Bayesian Best-Arm Identification
Source: arXiv:1910.10945 source file (2019-10-28)
Supplement: Supplementary file 2 [file app_optimal_weight.tex]

\section{Existence and uniqueness of the optimal proportion vector}\label{app:optimal_weight}

\restateoptim*

\begin{proof}
We handle the existence and the uniqueness separately as below.
    ~\paragraph{Existence} For any arm $i\neq I^\star$, $C_i$ is a continuous function, so as to $\min_{i\neq I^\star} C_i$. According to the \emph{extreme value theorem}, function $\min_{i\neq I^\star} C_i(\beta,\cdot)$ must attain its maximum over $[0,1]^{K-1}$ which is compact. Suppose that $\bomega^\beta$ is a such maximizer. We thus have
    \[
        \Gamma_{\beta}^\star = \max_{\bomega:\omega_{I^\star}=\beta}\min_{i\neq I^\star} C_i(\beta,\omega_i) = \min_{i\neq I^\star} C_i(\beta,\omega_i^\beta).
    \]
    Let us assume that $\bomega^\beta$ does not verify the second condition, which means there exists some $j\neq I^\star$ such that
    \[
        C_j(\beta,\omega_i^\beta) > C_{i^\star}(\beta,\omega_{i^\star}^\beta),
    \]
    where $i^\star \eqdef \argmin_{i\neq I^\star} C_i(\beta,\omega_i^\beta)$.
    Now if we subtract a small quantity $\epsilon>0$, from $C_j(\beta,\omega_j^\beta)$, such that
    \[
    \epsilon \leq \frac{C_j(\beta,\omega_j^\beta)-C_{i^\star}(\beta,\omega_{i^\star}^\beta)}{2},
    \]
    and add $\epsilon/(K-2)$ to $C_i(\beta,\omega_i^\beta)$ for any $i\neq j,I^\star$, we would not change the order of the $C_i(\beta,\omega_i^\beta)$. Therefore, $i^\star$ remains unchanged, however, the new $C_{i^\star}(\beta,\omega_{i^\star}^\beta)$ would be strictly larger than the previous one which contradicts the definition of $\bomega^\beta$.

    ~\paragraph{Uniqueness} We now need to show that the solution is unique. Suppose that two different maximizers $\bomega$ and $\bomega'$ exist, and there exists some $i\neq I^\star$ such that $\omega_i > \omega'_i$. Since $C_i(\beta,\cdot)$ is an strictly increasing function, thus we have $C_i(\beta,\omega_i)>C_i(\beta,\omega'_i)$. By consequence, for any $j\neq i$ and $j'\neq i$,
    \[
        C_j(\beta,\omega_j) = C_i(\beta,\omega_i) > C_i(\beta,\omega'_i) = C_{j'}(\beta,\omega'_{j'}).
    \]
    Therefore, for any $j\neq I^\star$ and $j'\neq I^\star$, $\omega_j > \omega'_j$, and
    \[
        \sum_{j\neq I^\star} \omega_j > \sum_{j\neq I^\star} \omega'_j.
    \]
    However, we know that $1-\sum_{j\neq I^\star} \omega_j = \omega_{I^\star} =  \beta = \omega'_{I^\star} = 1-\sum_{j\neq I^\star} \omega'_j$, contradiction!
\end{proof}
