# Supplementary material for: Fixed-Confidence Guarantees for Bayesian Best-Arm Identification
Source: arXiv:1910.10945 source file (2019-10-28)
Supplement: Supplementary file 3 [file app_pac_gaussian.tex]

\section{Proof of \texorpdfstring{$\delta$-}{}correctness}\label{app:pac_gaussian}

We hereby demonstrate Theorem~\ref{thm:pac_gaussian}. 

\restatepac*

For that purpose, we need the Gaussian tail inequality of Lemma~\ref{lemma:gaussiantails}. Now recall that what we want to show is that for a given $\delta\in (0,1)$,
\begin{equation*}
    \underbrace{\PP{\tau_{\delta} < \infty, J_{\tau_{\delta}}^{(1)} \neq I^\star}}_\text{(*)} \leq \delta
\end{equation*}
for a certain threshold $c_{n,\delta}$ to be determined.

\begin{proof}
Using the union bound, we have
\begin{align*}
\begin{split}
    \text{(*)} &= \PP{\bigcup_{i\neq I^\star} \left\{ \tau_{\delta} < \infty, J_{\tau_{\delta}}^{(1)} = i \right\}} \\
                  &\leq \sum_{i\neq I^\star} \PP{\tau_{\delta} < \infty, J_{\tau_{\delta}}^{(1)} = i} \\
                  &= \sum_{i\neq I^\star} \PP{\exists t \in \NN, a_{t,i} \geq c_{t,\delta}}.
\end{split}
\end{align*}

%We can be more precise on $a_{n,i}$. As we already stated in the main text, under improper priors with $\mu_{1,i}=0$ and $\sigma_{1,i}=+\infty$ for any $i\in\cA$, it is easy to compute the true posterior mean (which is identical to the empirical mean) and the posterior variance,
%\[
%    \mu_{n,i} = \hat{\mu}_{n,i} = \frac{1}{T_{n,i}} \sum_{l=1}^{n-1} \1\{I_l = i\}Y_{l,I_l}, \sigma_{n,i}^2 = \frac{\sigma^2}{T_{n,i}},
%\]
%and the posterior distribution can be written as
%\[
%    \Pi_{n} = \bigotimes_{i=1}^{K} \cN\left( \mu_{n,i}, \frac{\sigma^2}{T_{n,i}} \right).
%\]

%Therefore $\forall i\in\cA$ and $n\in\NN$,
%\begin{align*}
%\begin{split}
%    a_{n,i} &= \mathbb{P}_{\btheta\sim\Theta}\left[\theta_i > \max_{j\neq i} \theta_j \right] \\
%                 &= \int_{\Theta_i} \prod_{i=1}^{K} \frac{1}{\sqrt{2\pi}\sigma^2/T_{n,i}} \expp{-\frac{(\theta_i-\mu_{n,i})^2}{2\sigma^2/T_{n,i}}} d\btheta \\
%                 &= \int_{\Theta_i} \frac{1}{(\sqrt{2\pi}\sigma^2/T_{n,i})^K} \expp{-\sum_{i=1}^K\frac{(\theta_i-\mu_{n,i})^2}{2\sigma^2/T_{n,i}}} d\btheta. \\
%\end{split}
%\end{align*}

%The previous form is closely related to that of Conjecture Lemma~\ref{lemma:posterior}, since in the Gaussian case, $d(\mu_i;\theta_i) = \frac{(\theta_i-\mu_i)^2}{2\sigma^2}$.

At the end of round $n$, the algorithm would choose a wrong arm if there exists $i\neq I^\star$, s.t.
\[
	a_{n,i} \geq c_{n,\delta},
\]
which implies in particular,
\begin{equation}\label{eq:error}
	\Pi_{n}\left[\theta_i \geq \theta_{I^\star} \right] \geq c_{n,\delta}.
\end{equation}

The threshold $c_{n,\delta}$ is a large number ($>1/2$), thus the wrong pick could only occur if the posterior mean of arm $i$ is larger than the posterior mean of the true best arm $I^\star$,
\[
    \mu_{n,i} \geq \mu_{n,I^\star}.
\]
We are then prepared to apply Lemma~\ref{lemma:gaussiantails}. Since we have
\begin{align*}
    (\ref{eq:error}) &\iff 1 - \Pi_{n}\left[\theta_i < \theta_{I^\star} \right] \geq c_{n,\delta} \\
                     &\iff 1 - c_{n,\delta} \geq \Pi_{n}\left[\theta_i - \theta_{I^\star} < 0 \right] \\
\end{align*}
and rewriting $\Pi_{n}\left[\theta_i - \theta_{I^\star} < 0 \right]$ as 
\[
\Pi_{n}\left[\theta_i - \theta_{I^\star} < \mu_{n,i} - \mu_{n,I^\star} + \mu_{n,I^\star} - \mu_{n,i} \right],
\]
then applying Lemma~\ref{lemma:gaussiantails} with $c = \mu_{n,I^\star} - \mu_{n,i} \leq 0$, we obtain
\begin{align*}
    1 - c_{n,\delta} &\geq \frac{1}{\sqrt{2\pi}} \expp{-\frac{1}{2\sigma_{n,i,I^\star}^2}\left( \sigma_{n,i,I^\star}+\mu_{n,i}-\mu_{n,I^\star} \right)^2},
\end{align*}
where $\sigma_{n,i,I^\star} \eqdef \sqrt{\sigma^2/T_{n,i}+\sigma^2/T_{n,I^\star}}$. Hence, we have
\[
    \ln{\frac{1}{\sqrt{2\pi}(1-c_{n,\delta})}} \leq \frac{1}{2\sigma_{n,i,I^\star}^2}\left( \sigma_{n,i,I^\star}+\mu_{n,i}-\mu_{n,I^\star} \right)^2.
\]
We take square root of both sides since we know how to control $(\mu_{n,i}-\mu_{n,I^\star})^2/(2\sigma_{n,i,I^\star}^2)$, 
\[
    \sqrt{\ln{\frac{1}{\sqrt{2\pi}(1-c_{n,\delta})}}} - \frac{1}{\sqrt{2}} \leq \frac{1}{\sqrt{2}\sigma_{n,i,I^\star}} (\mu_{n,i}-\mu_{n,I^\star}),
\]
and finally,
\[
    \left( \sqrt{\ln{\frac{1}{\sqrt{2\pi}(1-c_{n,\delta})}}} - \frac{1}{\sqrt{2}} \right)^2 \leq \frac{(\mu_{n,i}-\mu_{n,I^\star})^2}{2\sigma_{n,i,I^\star}^2},
\]

Now we need to bound $(\mu_{n,i}-\mu_{n,I^\star})^2/(2\sigma_{n,i,I^\star}^2)$. We know that
\begin{align*}
    \frac{(\mu_{n,i}-\mu_{n,I^\star})^2}{2\sigma_{n,i,I^\star}^2} &= \inf_{\theta_i<\theta_{I^\star}} T_{n,i}d(\mu_{n,i};\theta_i) + T_{n,I^\star}d(\mu_{n,I^\star};\theta_{I^\star}),
\end{align*}
and using a result in Theorem 10 of~\citet{garivier2016tracknstop}, we know that if $\mu_{n,i} \geq \mu_{n,I^\star}$, then for any $\delta>0$,
\[
    \PP{\exists n\in\NN, \frac{(\mu_{n,i}-\mu_{n,I^\star})^2}{2\sigma_{n,i,I^\star}^2} > \ln{\frac{2n(K-1)}{\delta}}} \leq \frac{\delta}{K-1}.
\]
Note that the statistic $Z_n$ used by~\citet{garivier2016tracknstop} is exactly equal to $\inf_{\theta_i<\theta_{I^\star}} T_{n,i}d(\mu_{n,i};\theta_i) + T_{n,I^\star}d(\mu_{n,I^\star};\theta_{I^\star})$ in our Gaussian case.

Now denoting $\kappa_{n,\delta} \eqdef \left( \sqrt{\ln(1/(\sqrt{2\pi}(1-c_{n,\delta})))} - 1/\sqrt{2} \right)^2$, it suffices to set $\kappa_{n,\delta}$ to be equal to $\ln{2n(K-1)/\delta}$ so that for any $\delta > 0$,
\begin{align*}
\begin{split}
    \text{(*)} &\leq \sum_{i\neq I^\star} \PP{\exists t \in \NN, a_{t,i} \geq c_{t,\delta}} \\
    &\leq \sum_{i\neq I^\star} \PP{\exists t \in \NN, \frac{(\mu_{t,i}-\mu_{t,I^\star})^2}{2\sigma_{t,i,I^\star}^2} \geq \kappa_{t,\delta}} \\
    &\leq (K-1)\max_{i\neq I^\star} \PP{\exists t \in \NN, \frac{(\mu_{t,i}-\mu_{t,I^\star})^2}{2\sigma_{t,i,I^\star}^2} \geq \kappa_{t,\delta}} \\
    &\leq \delta.
\end{split}
\end{align*}
\end{proof}

By a simple computation, it suffices to set the threshold as
\[
    c_{n,\delta} \eqdef 1 - \ddfrac{\delta}{2n(K-1)\sqrt{2\pi e}\expp{\sqrt{2\ln{\frac{2n(K-1)}{\delta}}}}}
\]
to make sure that for any $\delta > 0$, $\PP{\tau_{\delta} < \infty, J_{\tau_{\delta}}^{(1)} \neq I^\star} \leq \delta$.

The previous result can be further refined since $\inf_{\theta_i<\theta_{I^\star}} T_{n,i}d(\mu_{n,i};\theta_i) + T_{n,I^\star}d(\mu_{n,I^\star};\theta_{I^\star})$ can be precisely bounded by $T_{n,i}d(\mu_{n,i};\mu_i) + T_{n,I^\star}d(\mu_{n,I^\star};\mu_{I^\star})$. (Apply for example Corollary 10 by~\citealt{kaufmann2018mixture}.)
