# Supplementary material for: Fixed-Confidence Guarantees for Bayesian Best-Arm Identification
Source: arXiv:1910.10945 source file (2019-10-28)
Supplement: Supplementary file 4 [file app_rate.tex]

\section{Computation of the optimal error decay rate}\label{app:rate}

In this section, we first describe how to approximate $\Gamma_{\beta}^\star$ under any prior of 1-dimensional exponential family. We then also provide a way to compute numerically $\Gamma_{\beta}^\star$ under Gaussian prior since it can be computed more explicitly.

\subsection{General case}

For any $i\neq I^\star$, $C_i(\beta,\omega_i)$ is defined as the output to a convex minimization problem for whom the unique solution has an analytic expression
\[
    \frac{\beta}{\beta+\omega_i}\mu_{I^\star} + \frac{\omega_i}{\beta+\omega_i}\mu_i.
\]
Next, we define for any $i\neq I^\star$, a function
\begin{align*}
  g_i \colon [0,+\infty[ &\to [0,+\infty[\\
  x &\mapsto \beta d\left(\mu_{I^\star};\frac{\beta}{\beta+\omega_i}\mu_{I^\star} + \frac{\omega_i}{\beta+\omega_i}\mu_i\right) + x d\left(\mu_i;\frac{\beta}{\beta+\omega_i}\mu_{I^\star} + \frac{\omega_i}{\beta+\omega_i}\mu_i\right).
\end{align*}
In fact, $g_i$ is a strictly increasing function (see~\citealt{garivier2016tracknstop}, Appendix A.2 for more details), so does its inverse function $x_i \eqdef g_i^{-1}$ which is defined on $[0, \beta d(\mu_{I^\star};\mu_i)[$ as $g_i$ tends to 0 when $x$ tends to 0 and tends to $\beta d(\mu_{I^\star};\mu_i)$ when $x$ tends to $+\infty$.

According to Proposition~\ref{prop:optim}, the optimal proportion vector $\bomega^\beta$ that we are searching for satisfies the constraint that $\forall i,j\neq I^\star$,
\[
    g_i(\omega_i^\beta) = g_j(\omega_j^\beta) = \Gamma_{\beta}^\star.
\]
Since $\omega_i^\beta = g_i^{-1}(\Gamma_{\beta}^\star) = x_i(\Gamma_{\beta}^\star)$, and we know that $\sum_{i\neq I^\star} \omega_i = 1-\beta$, thus the problem of computing $\Gamma_{\beta}^\star$ is equivalent to solve the following equation,
\[
    \sum_{i\neq I^\star} x_i(y) = 1 - \beta.
\]
This equation has a unique solution since $\sum_{i\neq I^\star}$ is a strictly increasing function valued in $[0, +\infty[$. We can thus apply a bisection method to this function whose evaluation require itself a bisection method applied on $K-1$ smooth scalar functions.

\subsection{Gaussian case}

In the context of this paper, we can do a more efficient approximation. In the Gaussian case, we know that for any $i,j\neq I^\star$,
\[
    \frac{1}{\omega_j^\beta} + \frac{1}{\beta} = \frac{(\mu_{I^\star}-\mu_j)^2}{(\mu_{I^\star}-\mu_i)^2}\left(\frac{1}{\omega_i^\beta} + \frac{1}{\beta}\right).
\]
Denote $x_i\eqdef 1/\omega_i^\beta+1/\beta$ and $a_{ji}\eqdef (\mu_{I^\star}-\mu_j)^2/(\mu_{I^\star}-\mu_i)^2$, fix some $i\neq I^\star$, then we have $\forall j\neq I^\star$, $x_j = a_{ji}x_i$. Since $\sum_{j\neq I^\star} \omega_j^\beta = 1-\beta$, we have
\[
    \sum_{j\neq I^\star} \frac{1}{x_j-1/\beta} = \sum_{j\neq I^\star} \frac{1}{a_{ji}x_i-1/\beta} = 1-\beta.
\]
Thus we only need to find the unique solution to the equation
\[
    \sum_{j\neq I^\star} \frac{a_{ij}}{x-a_{ij}/\beta} = 1-\beta,
\]
that requires only one shot bisection method.
